# Supplementary material for: Basins of Attraction, Commitment Sets and Phenotypes of Boolean Networks
Source: arXiv:1807.10103 source file (2018-07-26)
Supplement: Supplementary file 1 [file klarner_basins_supp.pdf]

# Basins, Commitment Sets and Phenotypes of Boolean networks - Supplementary Materials

Hannes Klarner, Frederike Heinitz, Sarah Nee, Heike Siebert

May 7, 2018

## 1 CTL Model Checking

Model checking is a formal method from computer science to determine whether a transition system satisfies a temporal specification. See [1] for a review of its application to computational biology and [2] for an introduction to model checking.

A *transition system* is a 5-tuple  $TS = (S, \rightarrow, AP, L, I)$  where  $(S, \rightarrow)$  is a state transition graph,  $AP$  a set of atomic propositions,  $L : S \rightarrow 2^{AP}$  a labelling function and  $I \subseteq S$  a set of initial states. In its simplest form the atomic propositions  $AP := \{v = c \mid v \in V, c \in \mathbb{B}\}$  are used, where  $\mathbb{B} = \{0, 1\}$  is the set of Boolean values, and we define the labelling function  $L$  by

$$v = c \in L(x) :\Leftrightarrow x(v) = c$$

for all  $c \in \mathbb{B}$  and  $x \in S$ .

Queries in the Computation Tree Logic (CTL) language are built by recursively using quantified path operators and state formulas or by connecting two queries with the usual logical connectives. For this paper it is sufficient to define the following CTL fragment. A formula  $\varphi$  is defined by

$$\varphi ::= a \mid \varphi_1 \wedge \varphi_2 \mid \varphi_1 \vee \varphi_2 \mid \mathbf{EF}(\varphi) \mid \mathbf{EX}(\varphi) \mid \mathbf{AF}(\varphi) \mid \mathbf{AG}(\varphi)$$

where  $a \in AP$ . **EF** is the *exists finally* operator, **EX** is the *exists next* operator, **AF** is the *all finally* operator and **AG** the *always globally* operator. The intuition behind these operators is that, for example, **EF**( $\varphi$ ) is true in a state  $x \in S$  if there exists a path starting in  $x$  that satisfies  $\varphi$  at some point. We denote the set of paths starting in  $x$  by  $Paths(x)$  and write  $x \models \varphi$  to indicate that  $x$  satisfies  $\varphi$ . The semantics of the operators and the satisfaction relation  $\models$  for transition systems and CTL formulas are defined in Tab. 1.

## 2 Computational Cost of Commitment Diagram

How many model checks are required to construct the commitment diagram? In the worst case it contains all possible nodes and edges. There are  $2^k - 1$

**Table 1.** The satisfaction relation  $\models$  for CTL formulas  $\varphi$ , states  $x \in S$  and transition systems  $TS = (S, \rightarrow, Ap, L, I)$ .

|                                        |                    |                                                                                  |
|----------------------------------------|--------------------|----------------------------------------------------------------------------------|
| $x \models a$                          | $:\Leftrightarrow$ | $a \in L(x)$                                                                     |
| $x \models \varphi_1 \wedge \varphi_2$ | $:\Leftrightarrow$ | $x \models \varphi_1$ and $x \models \varphi_2$                                  |
| $x \models \varphi_1 \vee \varphi_2$   | $:\Leftrightarrow$ | $x \models \varphi_1$ or $x \models \varphi_2$                                   |
| $x \models \mathbf{EF}(\varphi)$       | $:\Leftrightarrow$ | $\exists \pi \in Paths(x) : \exists i \in \mathbb{N}_0 : \pi[i] \models \varphi$ |
| $x \models \mathbf{EX}(\varphi)$       | $:\Leftrightarrow$ | $\exists \pi \in Paths(x) : \pi[1] \models \varphi$                              |
| $x \models \mathbf{AF}(\varphi)$       | $:\Leftrightarrow$ | $\forall \pi \in Paths(x) : \exists i \in \mathbb{N}_0 : \pi[i] \models \varphi$ |
| $x \models \mathbf{AG}(\varphi)$       | $:\Leftrightarrow$ | $\forall \pi \in Paths(x) : \forall i \in \mathbb{N}_0 : \pi[i] \models \varphi$ |
| $TS \models \varphi$                   | $:\Leftrightarrow$ | $\forall x \in I : x \models \varphi$                                            |

nodes. For each of the  $\binom{k}{i}$  nodes  $C_T$  with  $|T| = i$  we have to perform  $2^i - 1$  model checks to decide whether the respective edge to a smaller commitment set exists. Note that  $k$  is a constant and  $i$  satisfies  $2 \leq i \leq k$ . The total number of model checks, in the worst case, for constructing a commitment diagram for a network with  $k$  attractors is therefore:

$$(2^k - 1) + \sum_{i=2}^k \binom{k}{i} (2^i - 1).$$

## References

- [1] Miguel Carrillo, Pedro A G3ngora, and David A Rosenblueth. An overview of existing modeling tools making use of model checking in the analysis of biochemical networks. *Frontiers in plant science*, 3, 2012.
- [2] Christel Baier and Joost-Pieter Katoen. *Principles of Model Checking*. The MIT Press, 2008.
